# Supplementary material for: Rethinking Dense Retrieval's Few-Shot Ability
Source: arXiv:2304.05845 source file (2023-04-12)
Supplement: Supplementary file 1 [file appendix.tex]

\section{Example Appendix}
\label{sec:appendix}

This is a section in the appendix.
